# Supplementary material for: Maximum Return on Investment for a Domestic Photovoltaic Installation
Source: arXiv:2310.09323 source file (2023-10-13)
Supplement: Supplementary file 1 [file appendix.tex]

\appendix
\chapter{First Appendix}
